# Supplementary material for: Efficient Random Phase Approximation for Diradicals
Source: arXiv:2404.18691 source file (2024-04-29)
Supplement: Supplementary file 1 [file SI_diradicals.pdf]

# Supporting Information for "Efficient Random Phase Approximation for Diradicals"

Reza G. Shirazi, Dmitry S. Golubev, Vladimir V. Rybkin, and Michael Marthaler

*HQS Quantum Simulations GmbH, Rintheimer Str. 23, 76131 Karlsruhe, Germany*

E-mail:

# Active orbitals for the test molecules

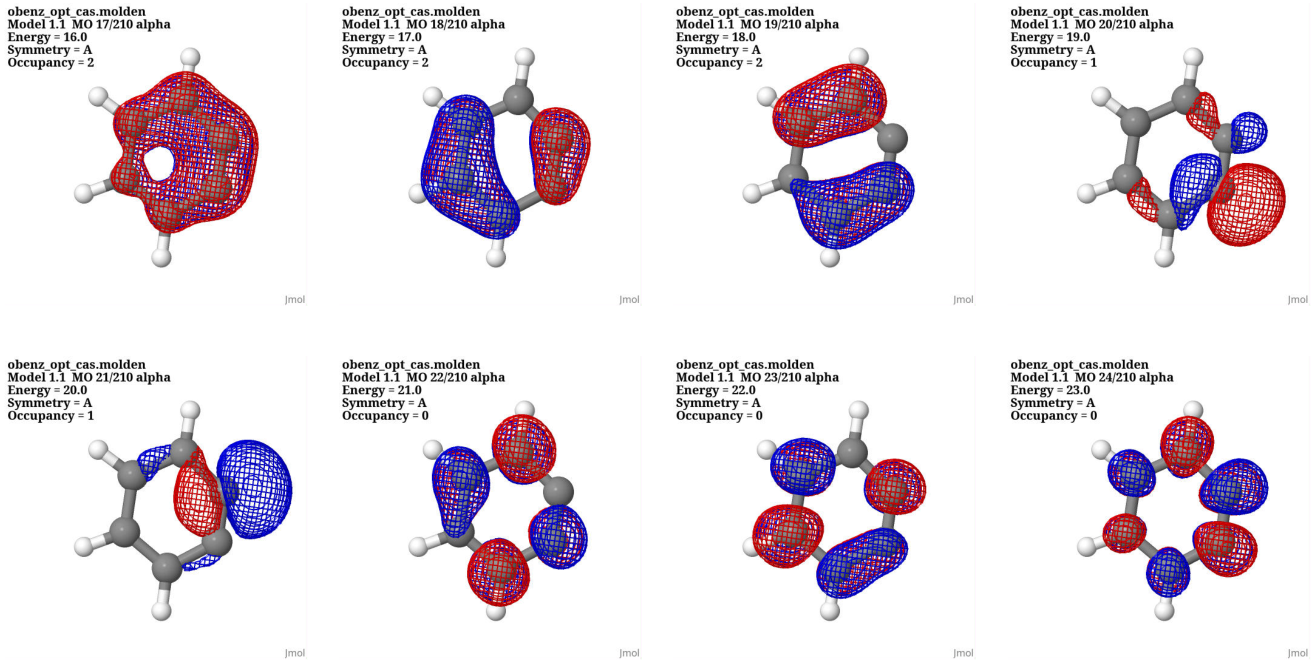


Figure 1: *o*-benzyne.

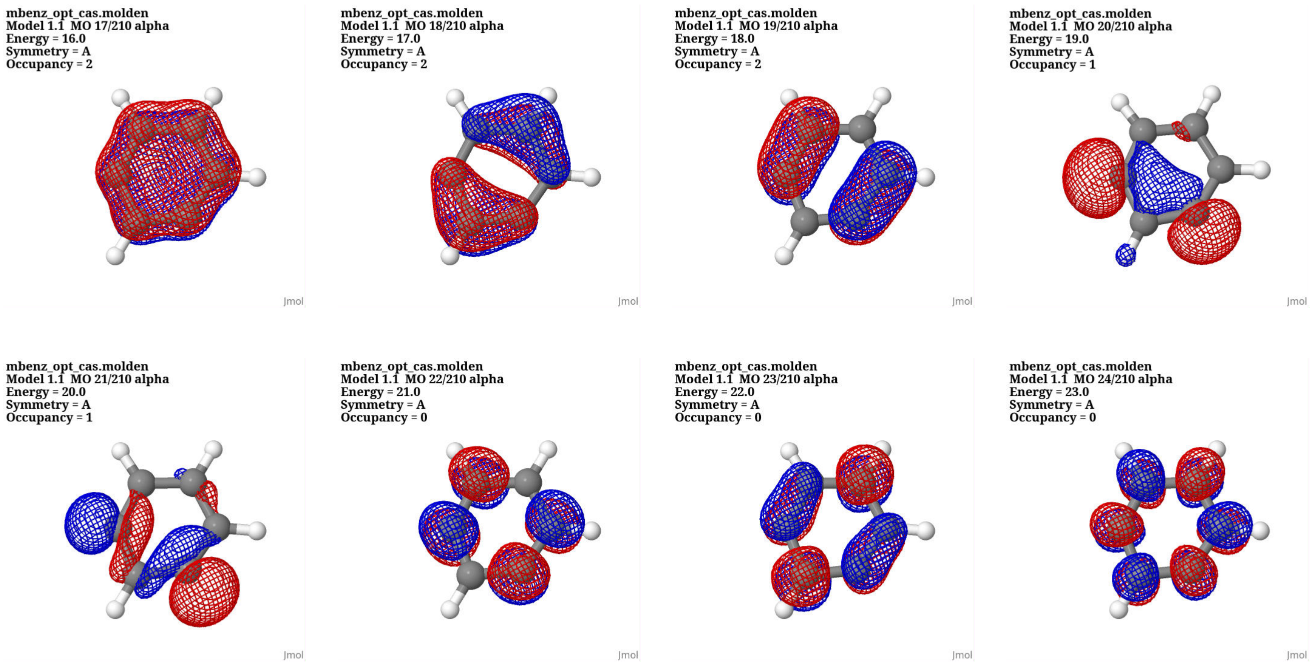


Figure 2: *m*-benzyne.

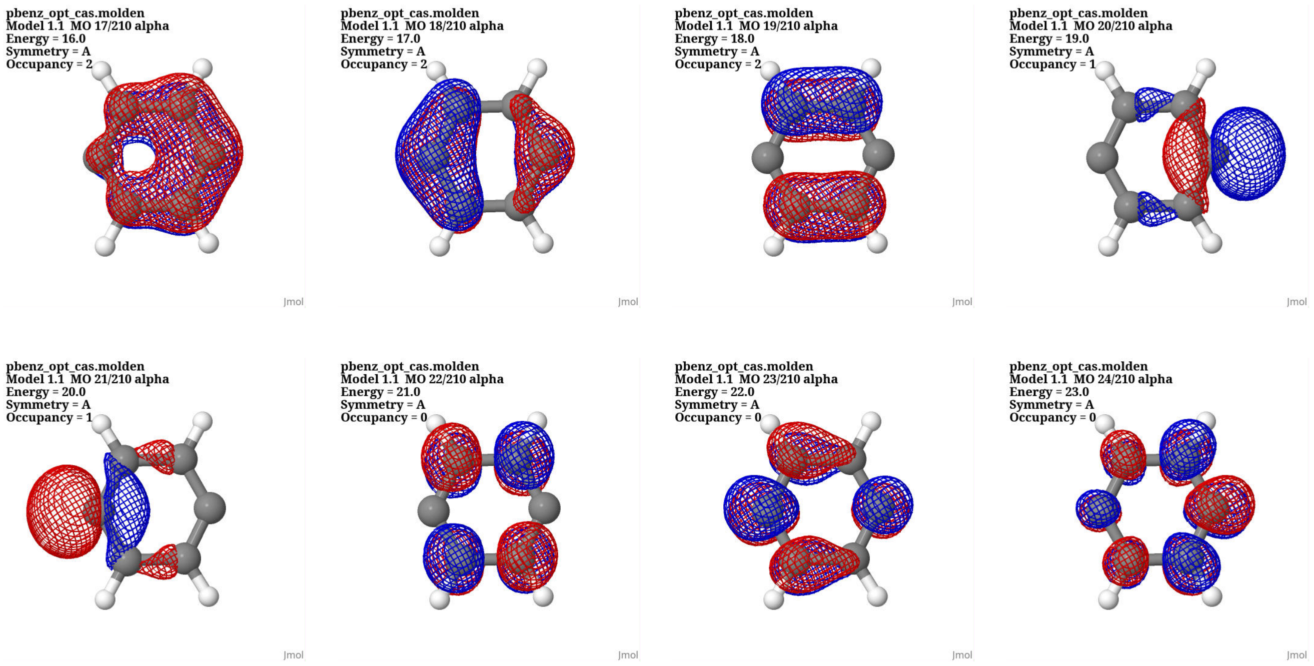


Figure 3: *p*-benzyne.

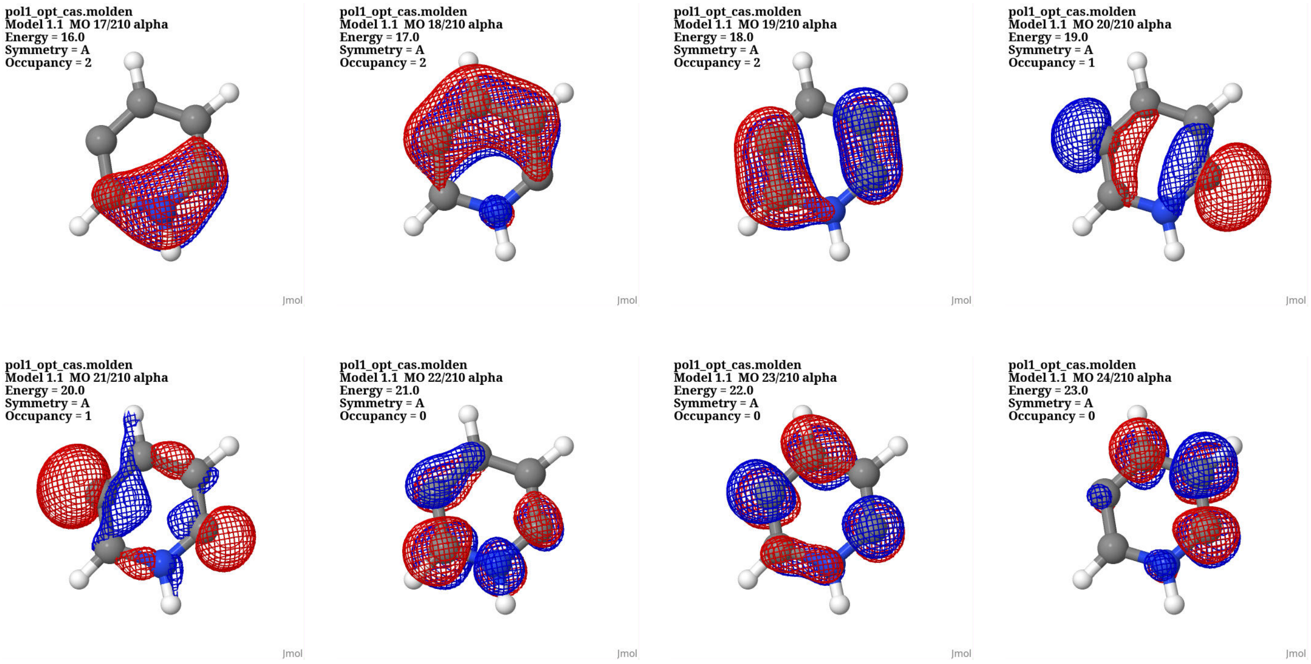


Figure 4: 2,5-didehydropyridinium cation (DDP-1).

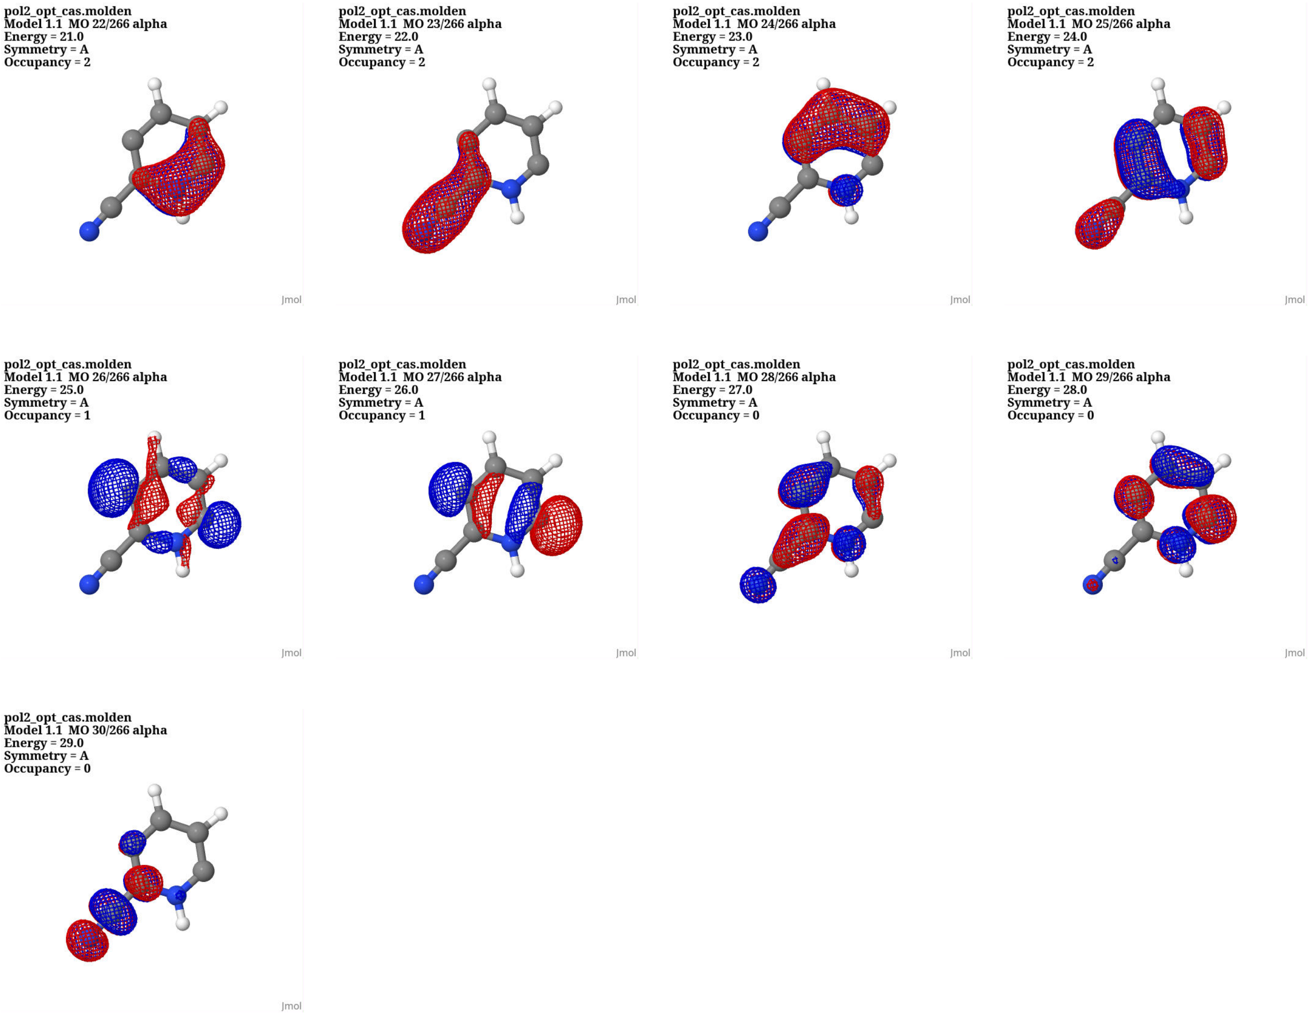


Figure 5: 6-cyano-2,5-didehydropyridinium cation (DDP2-2)

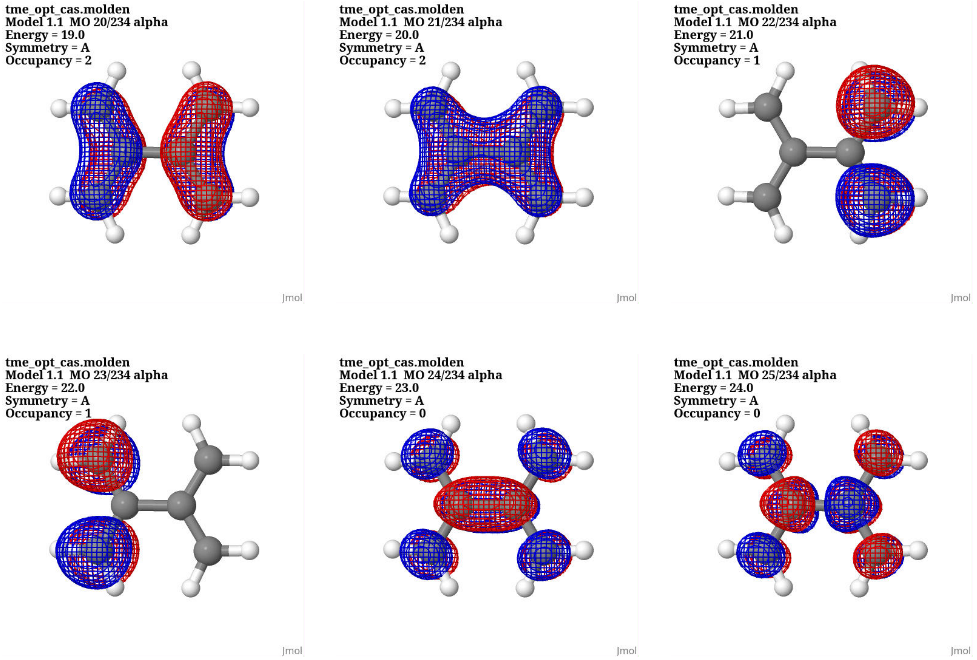


Figure 6: trimethylethylene (TME).

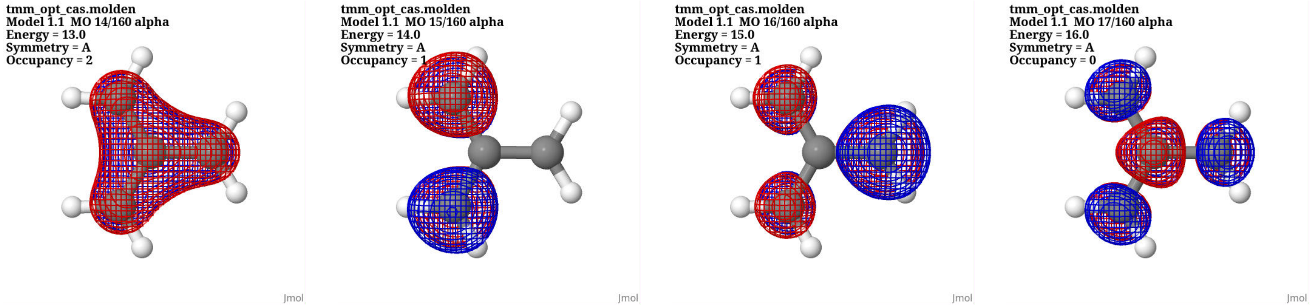


Figure 7: trimethylenemethane (TMM).

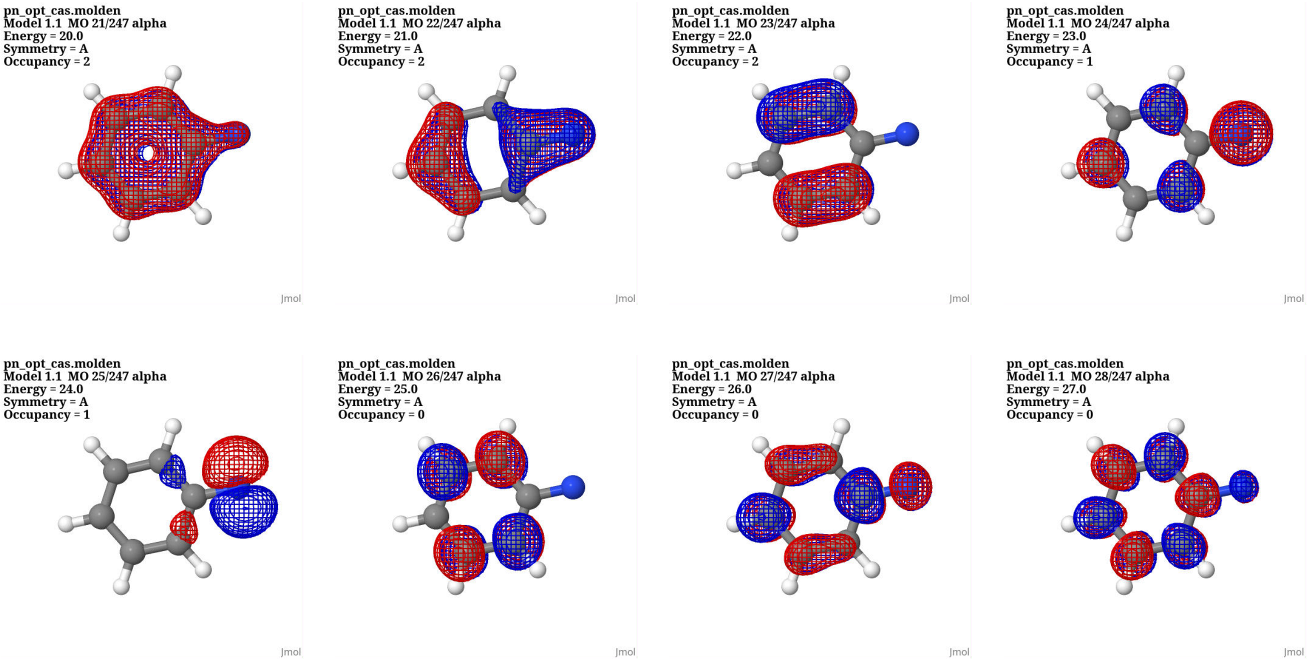


Figure 8: phenylnitrene (PN)

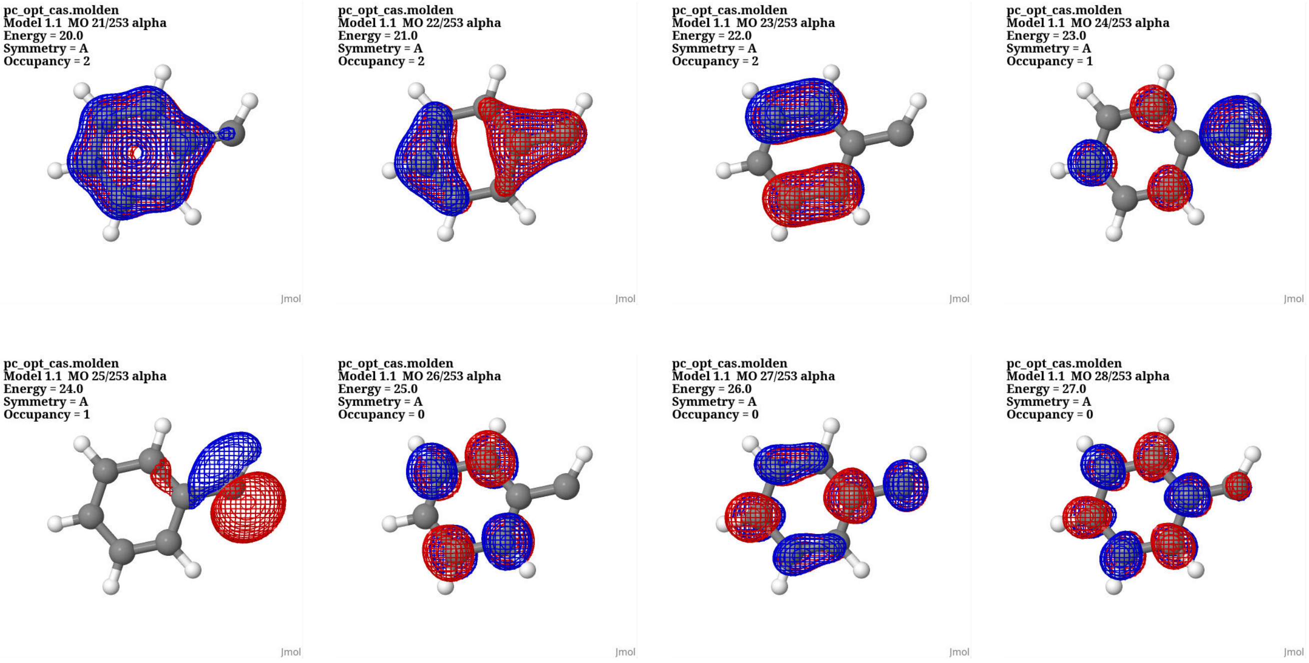


Figure 9: phenylcarbene (PC).

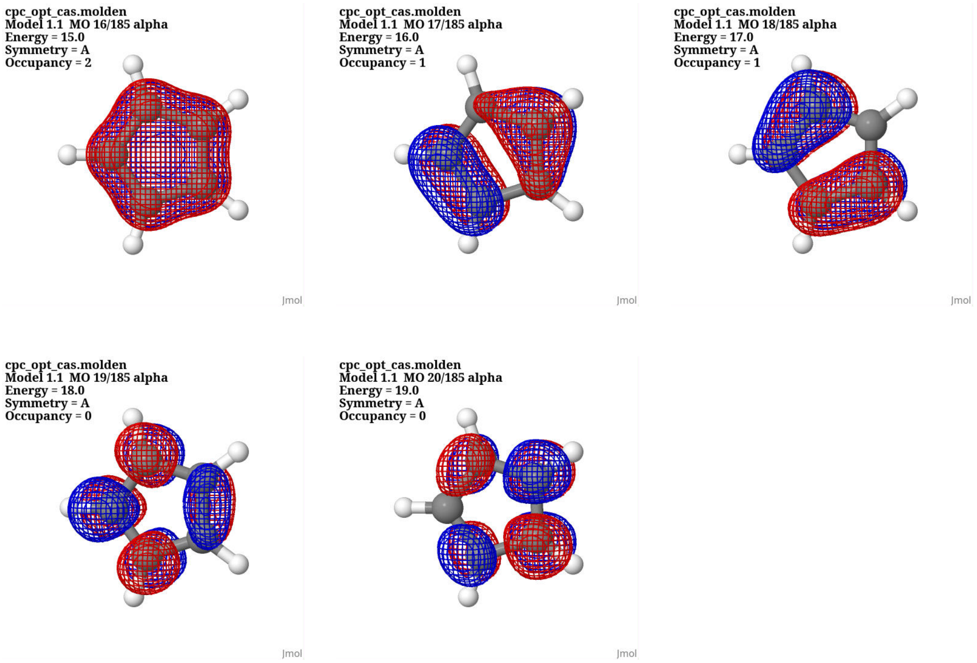


Figure 10: cyclopentane cation (CPC).
